# Supplementary material for: Measuring Human Perception to Improve Open Set Recognition
Source: arXiv:2209.03519 ancillary file (2023-04-24)
Supplement: Supplementary file 1 [file T_PAMI-2.pdf]

# Supplemental Material: Measuring Human Perception to Improve Open Set Recognition

## 1 Additional Details For the Psychophysical Study

### 1.1 Data Collection Process on Amazon Mechanical Turk

Here we provide some additional details about our data collection process, including screen shots for key steps. The data collection application is very user-friendly. Built with Python and Flask in the back-end and distributed on Amazon Mechanical Turk, the survey can be accessed simply using a web link.

**Directions**

**Overview**

This experiment will test your ability to find images that are same as reference images. Some of the questions asked will be easy, and others will be much harder. Do your best to answer correctly, taking as much time as is needed. You will be shown two rows of images. Be aware that in some cases not all images will appear, and the undisplayed ones will appear as broken image links. This is okay and the experiment is still working as intended.

**Description**

(1) In the first row, 5 images will be shown in a green box as your reference images.

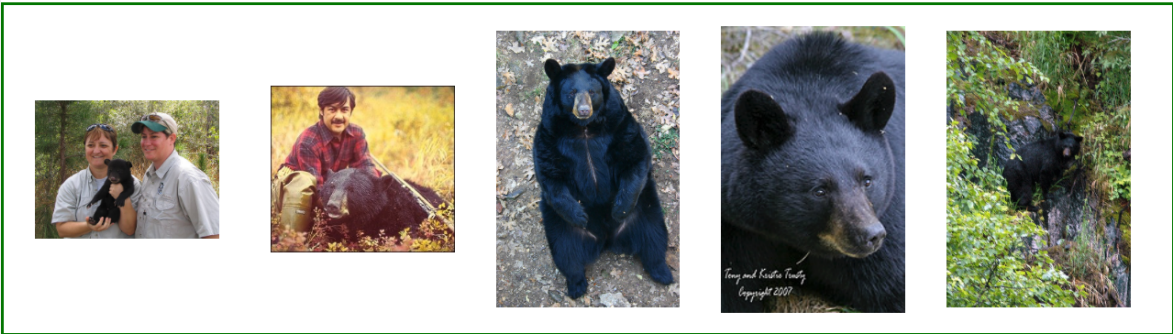

(2) In the bottom row, 5 images will be shown, labelled from 1 to 5. Your task will be to find the first image in the bottom row, when you look left to right, that belongs with those in the row above it. If you believe all 5 images show the same object type that is found in the top row, then you should select the sixth image, which shows the text: "There is no image that looks different from others".

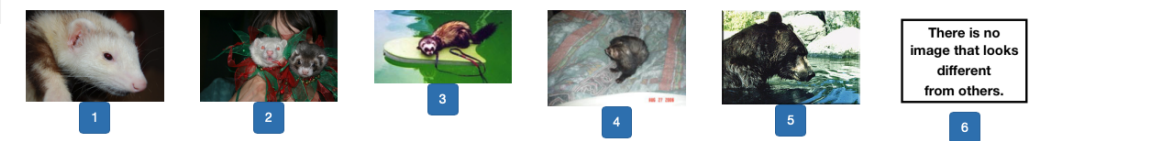

(3) What makes an image familiar is up to you to decide and may change depending on the group of images that are being tested. For example, four of the images in the bottom row above contain a bear while the 5th does not. It is possible that every once in a while, you will get a set that contains fewer than five images. Your task in this case is the same, but please only consider the images actually displayed. Feel free to zoom in on the images on the page if you need to check them more closely.

You may click the 1-5 buttons with your mouse pointer or press 1-5 on your keyboard

1 2

 or 

|           |   |   |   |    |   |
|-----------|---|---|---|----|---|
| ~         | ! | @ | # | \$ |   |
|           | 1 | 2 | 3 | 4  |   |
| Tab       | ← | Q | W | E  | R |
| Caps Lock | ↑ | A | S | D  |   |

Figure 1: Introductory page of each survey.

After a subject accesses the link, they first view an introductory page. This page includes following information:

1. Description, length and completion criteria. A brief overview about the survey, including the number of questions contained in each survey and what a subject is supposed to do to accomplish it, as well as what happens when a subject finishes answering all the questions.

2. Approval criteria and rejection criteria. In order to be approved, the subject needs to submit the survey code given at the end of a survey, as well as answer at least 3 control questions out of 5 correctly. A submission will be rejected if any of the following problems are present: (1) Failure to complete the survey. (2) Unable to provide a valid survey code. (3) Multiple submissions of an identical survey code. (4) 3 or more control questions are incorrect.
3. Troubleshooting guidelines. Information on what to do if an error shows up on the website is provided.

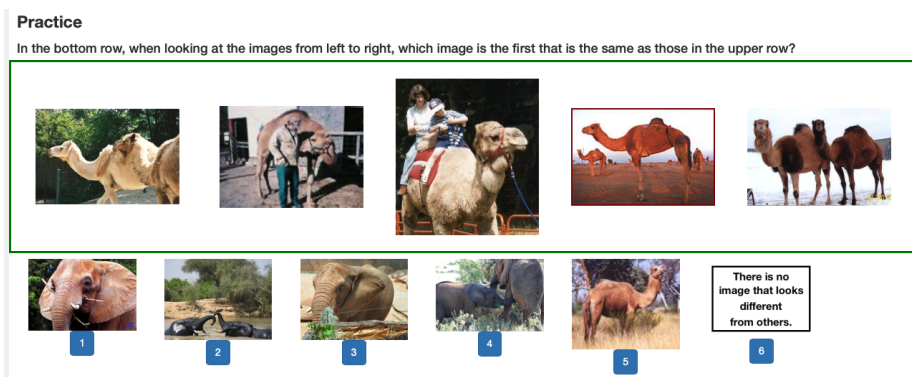

Figure 2: Practice question of a survey.

After the subject reads the introduction, the website proceeds to the consent page, where the subject is provided the information about the study, the purpose of the research, how long it takes to finish a survey, how to end a survey, how much we pay for a survey, and the privacy policy. The subject must check a box at the bottom of this page to agree to participate.

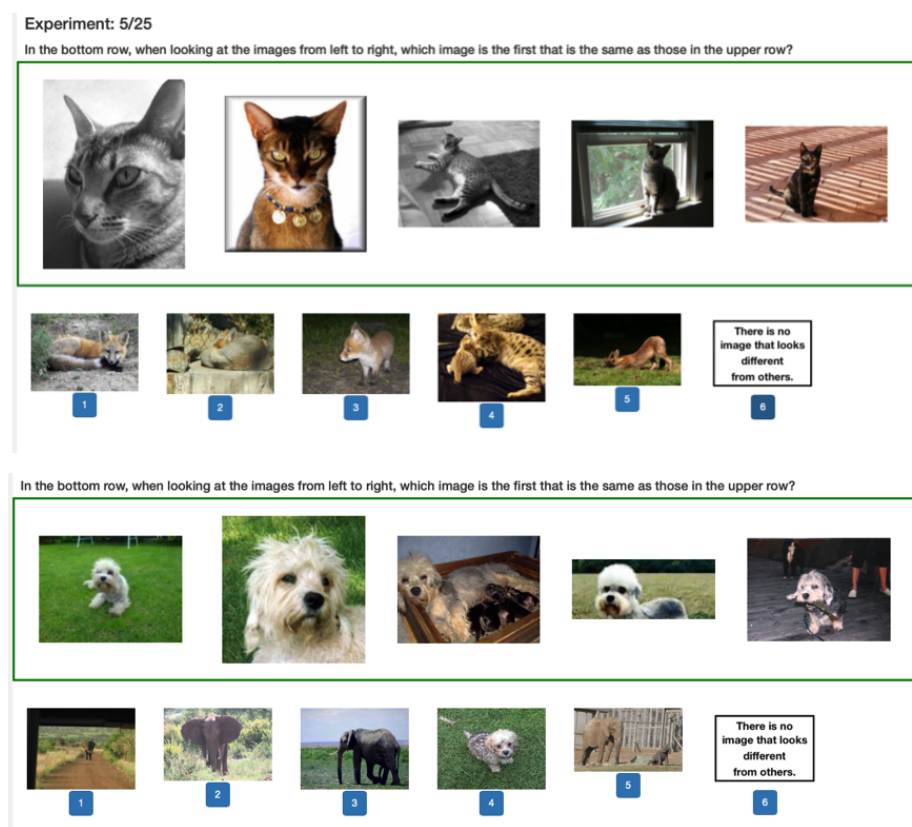

Figure 3: The different surveys vary in difficulty. The question at the top of this figure is more difficult because of the similarity between class cat and class fox; the question on the bottom of this figure is easier because of the large difference in visual appearance between dogs and elephants.

The survey then moves to the directions page as shown in Fig. 1. This page has an overview of the format of the questions that will appear in the survey, and it introduces the question format in detail: (1) showing the reference images in the top row in the green box. (2) showing the six options for selection in the bottom row. (3) giving direction on how to make a selection by either clicking on the buttons under an image or pressing a number key on a keyboard.

After the directions, the survey moves to a practice page that has a sample question (as shown in Fig. 2) to make sure that the subject understands how to answer the questions. The survey will only move forward to the real questions after this practice question is answered correctly.

For the actual data collection, 25 survey questions are presented to the subject, who will answer them as each question appears. Among all the questions, there are easier questions and harder questions, as shown in Fig. 3. After all of the questions are answered, a conclusion page will appear, and a survey code is provided for payment; an example of this is shown in Fig. 4

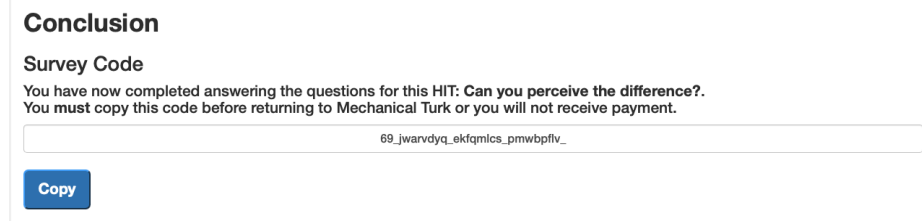

**Conclusion**

**Survey Code**

You have now completed answering the questions for this HIT: Can you perceive the difference?.  
You must copy this code before returning to Mechanical Turk or you will not receive payment.

69\_jwarvdyq\_ektqmics\_pmwbpfiv\_

**Copy**

Figure 4: Conclusion page with the survey code and instruction on submitting the code for payment.

## 1.2 Class-Level Reaction Time Analysis

Here we provide all the box plots for the class-level RT distributions for the 40 known classes used in the behavioral experiments. To understand these plots, consider the first one. In Fig. 5, the first figure shows the case when class 4 is used as the host class (the reference class / known class) and paired with other classes, which means all RTs are collected for class 4 specifically. Although the maximum RTs when paring with different classes vary by quite a bit, we can tell from the plot that the minimums, lower quartiles, and medians are rather close among all the class pairings. This observation indicates that class level RT will not provide useful additional information for supervised machine learning training. The same is true of the other 39 classes shown below. To make the figures easier to read and understand, Table 1 shows the mapping between class index from ImageNet335 and the names of these classes.

| Label | Class Name | Label | Class Name | Label | Class Name  | Label | Class Name  | Label | Class Name   |
|-------|------------|-------|------------|-------|-------------|-------|-------------|-------|--------------|
| 4     | cat        | 5     | black bear | 10    | giant panda | 11    | raccoon     | 55    | magpie       |
| 73    | butterfly  | 91    | flower     | 108   | sunglasses  | 114   | headset     | 115   | loud speaker |
| 133   | radiator   | 135   | switch     | 141   | organ       | 142   | piano       | 144   | drum         |
| 154   | candle     | 155   | spotlight  | 156   | neck brace  | 162   | scanner     | 163   | car mirror   |
| 164   | spider web | 171   | keyboard   | 172   | crane       | 173   | ski         | 202   | coffee mug   |
| 205   | barrel     | 206   | bathtub    | 207   | bucket      | 236   | staff       | 237   | drumstick    |
| 238   | spindle    | 273   | nest       | 274   | curtain     | 314   | fridge      | 315   | curling iron |
| 343   | theatre    | 286   | sweater    | 402   | menu        | 403   | bell pepper | 410   | gravel       |

Table 1: Label mapping for the class names of the 40 known classes.

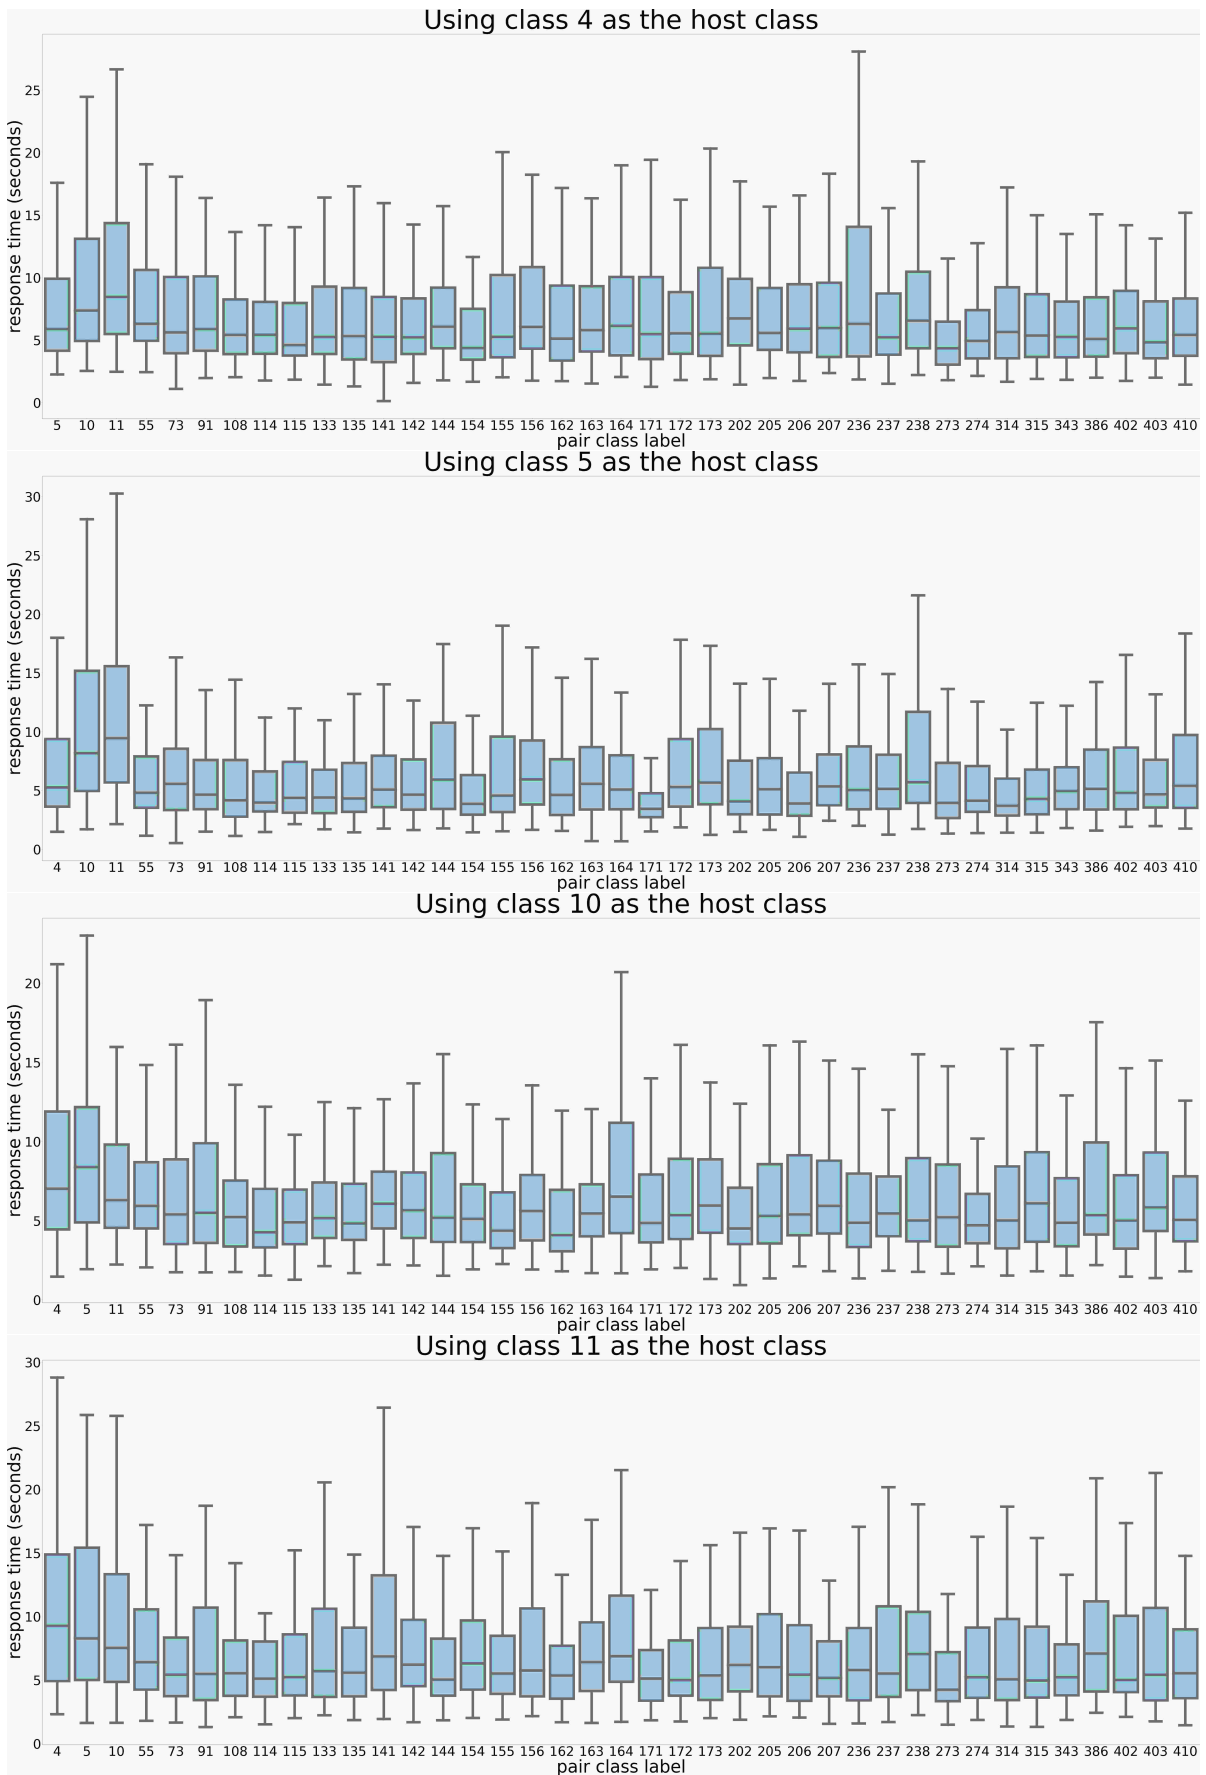

Figure 5: Using class 5, 10 and 11 as the host class

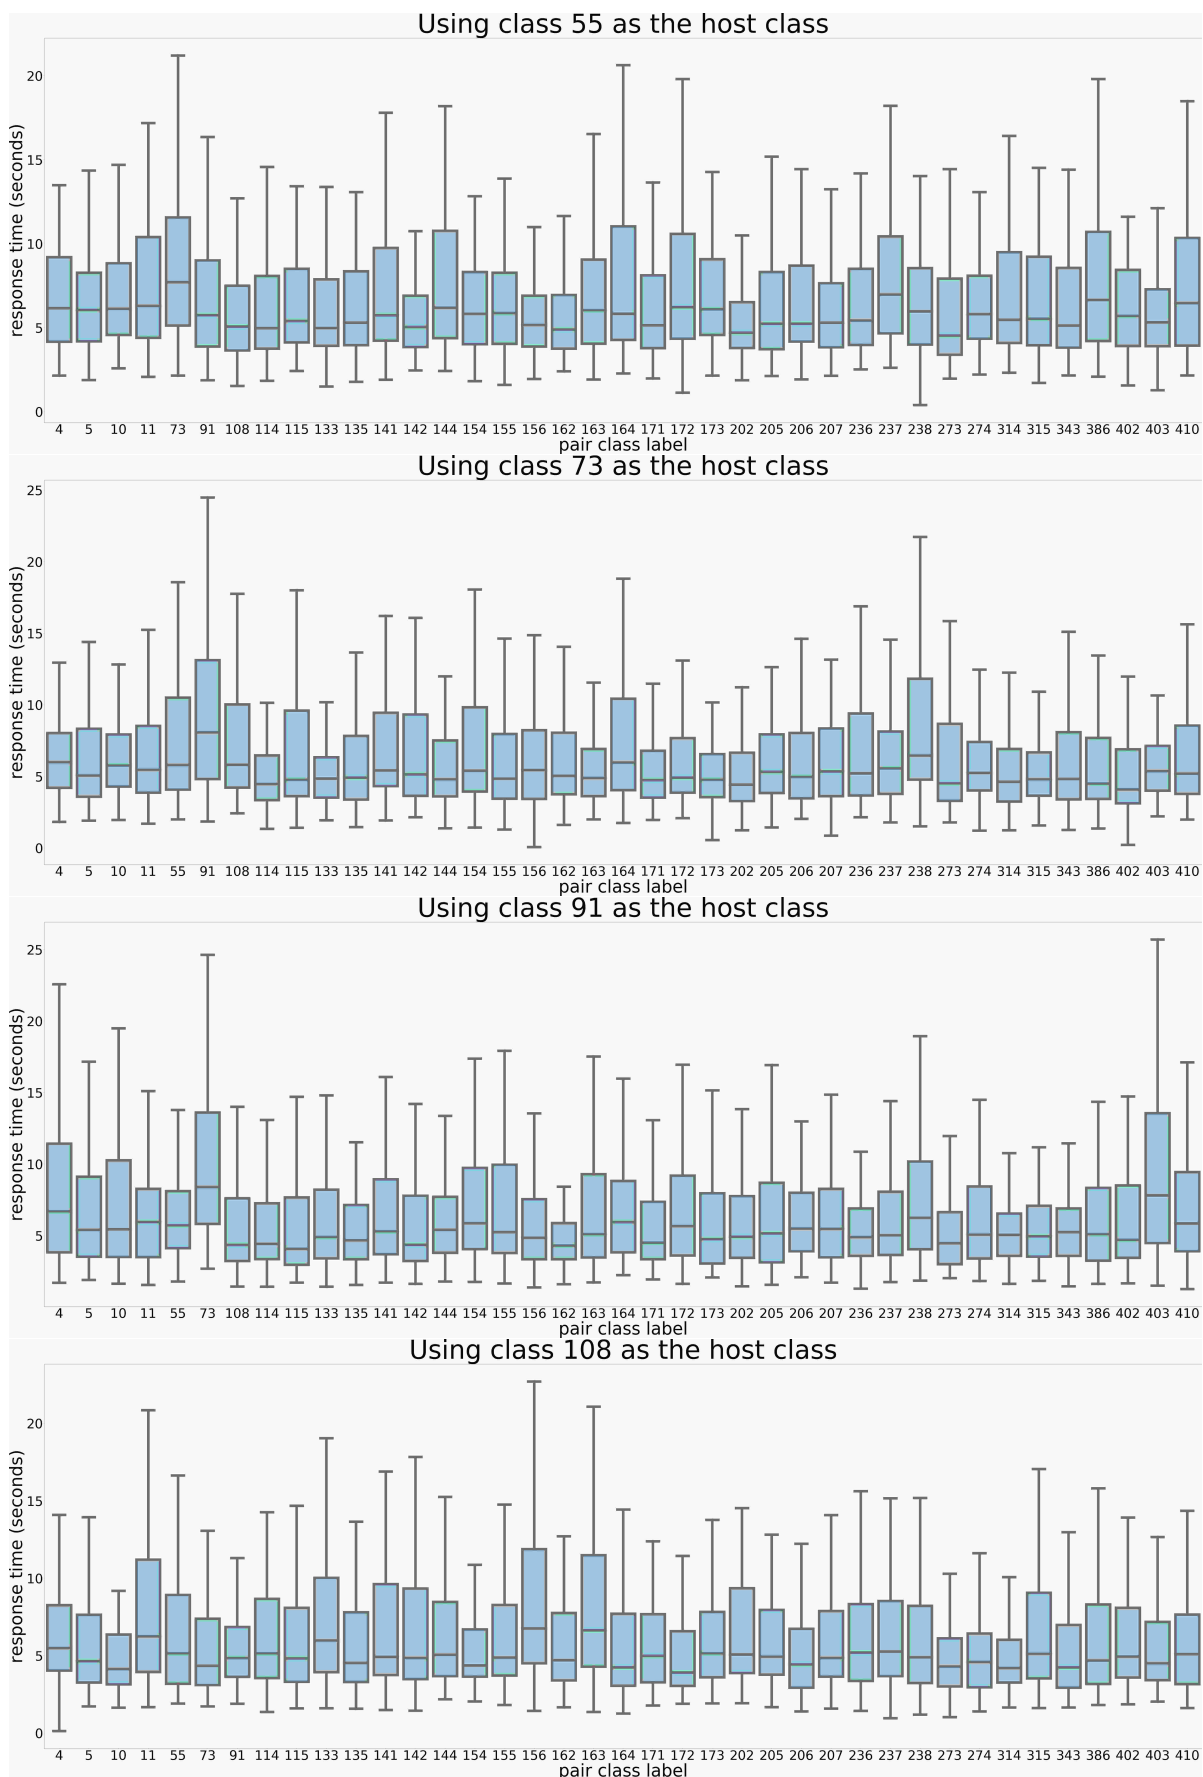

Figure 6: Using class 55, 73, 91 and 108 as the host class

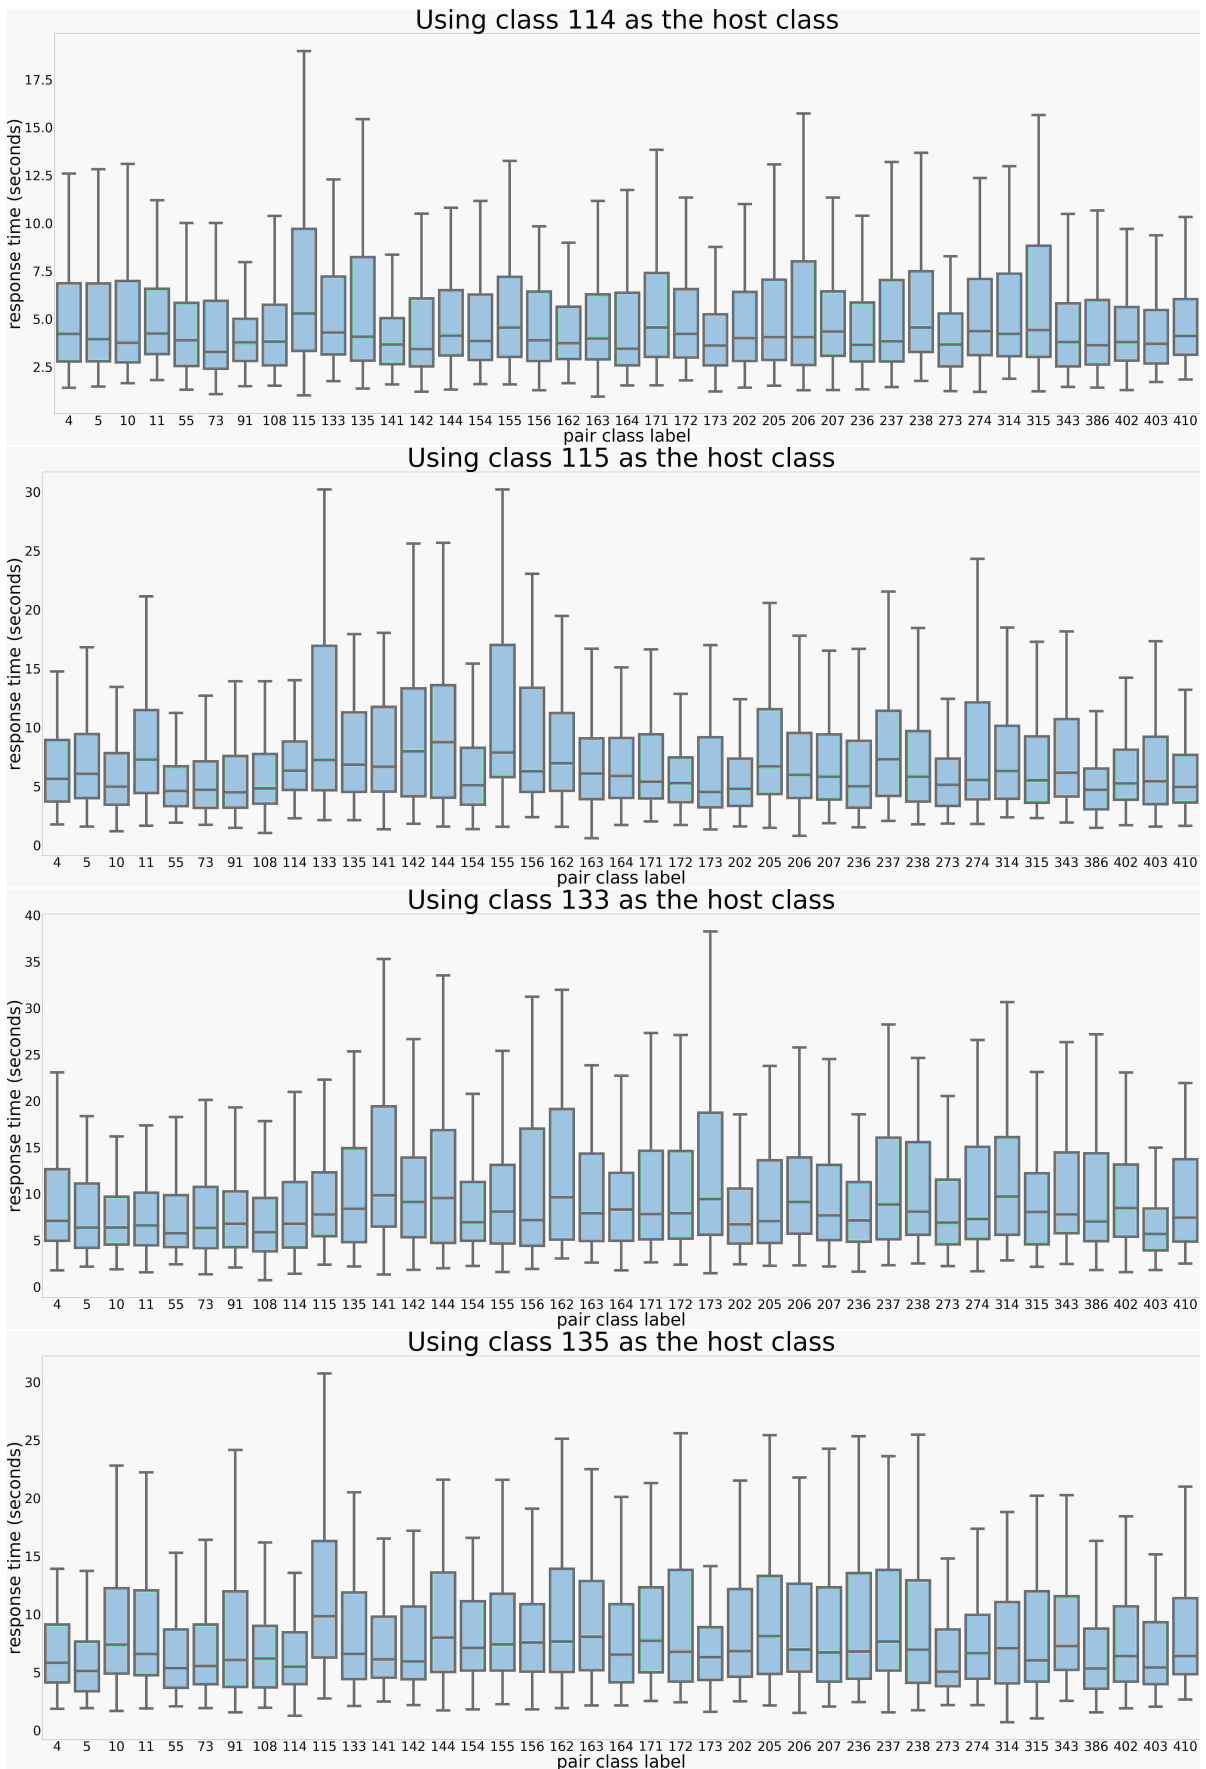

Figure 7: Using class 114, 115, 133 and 135 as the host class

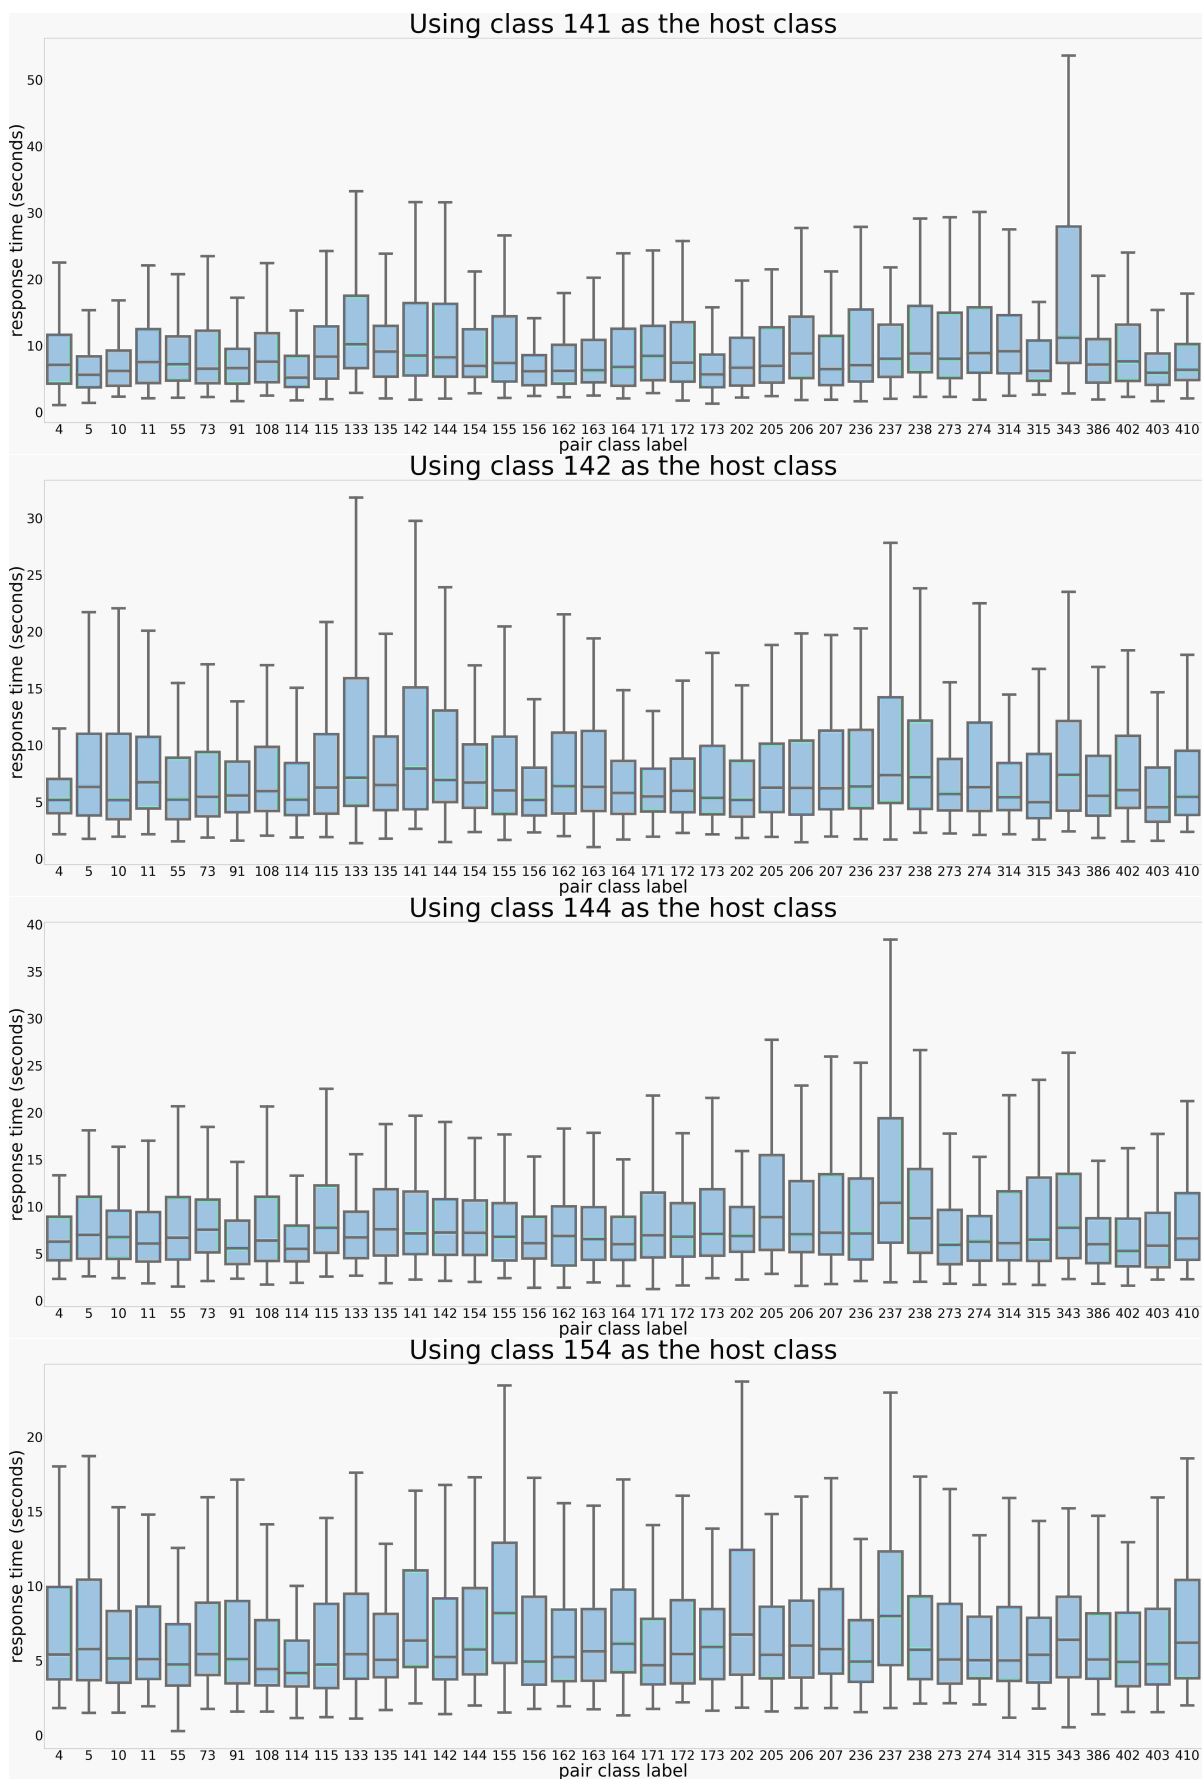

Figure 8: Using class 141, 142, 144 and 154 as the host class

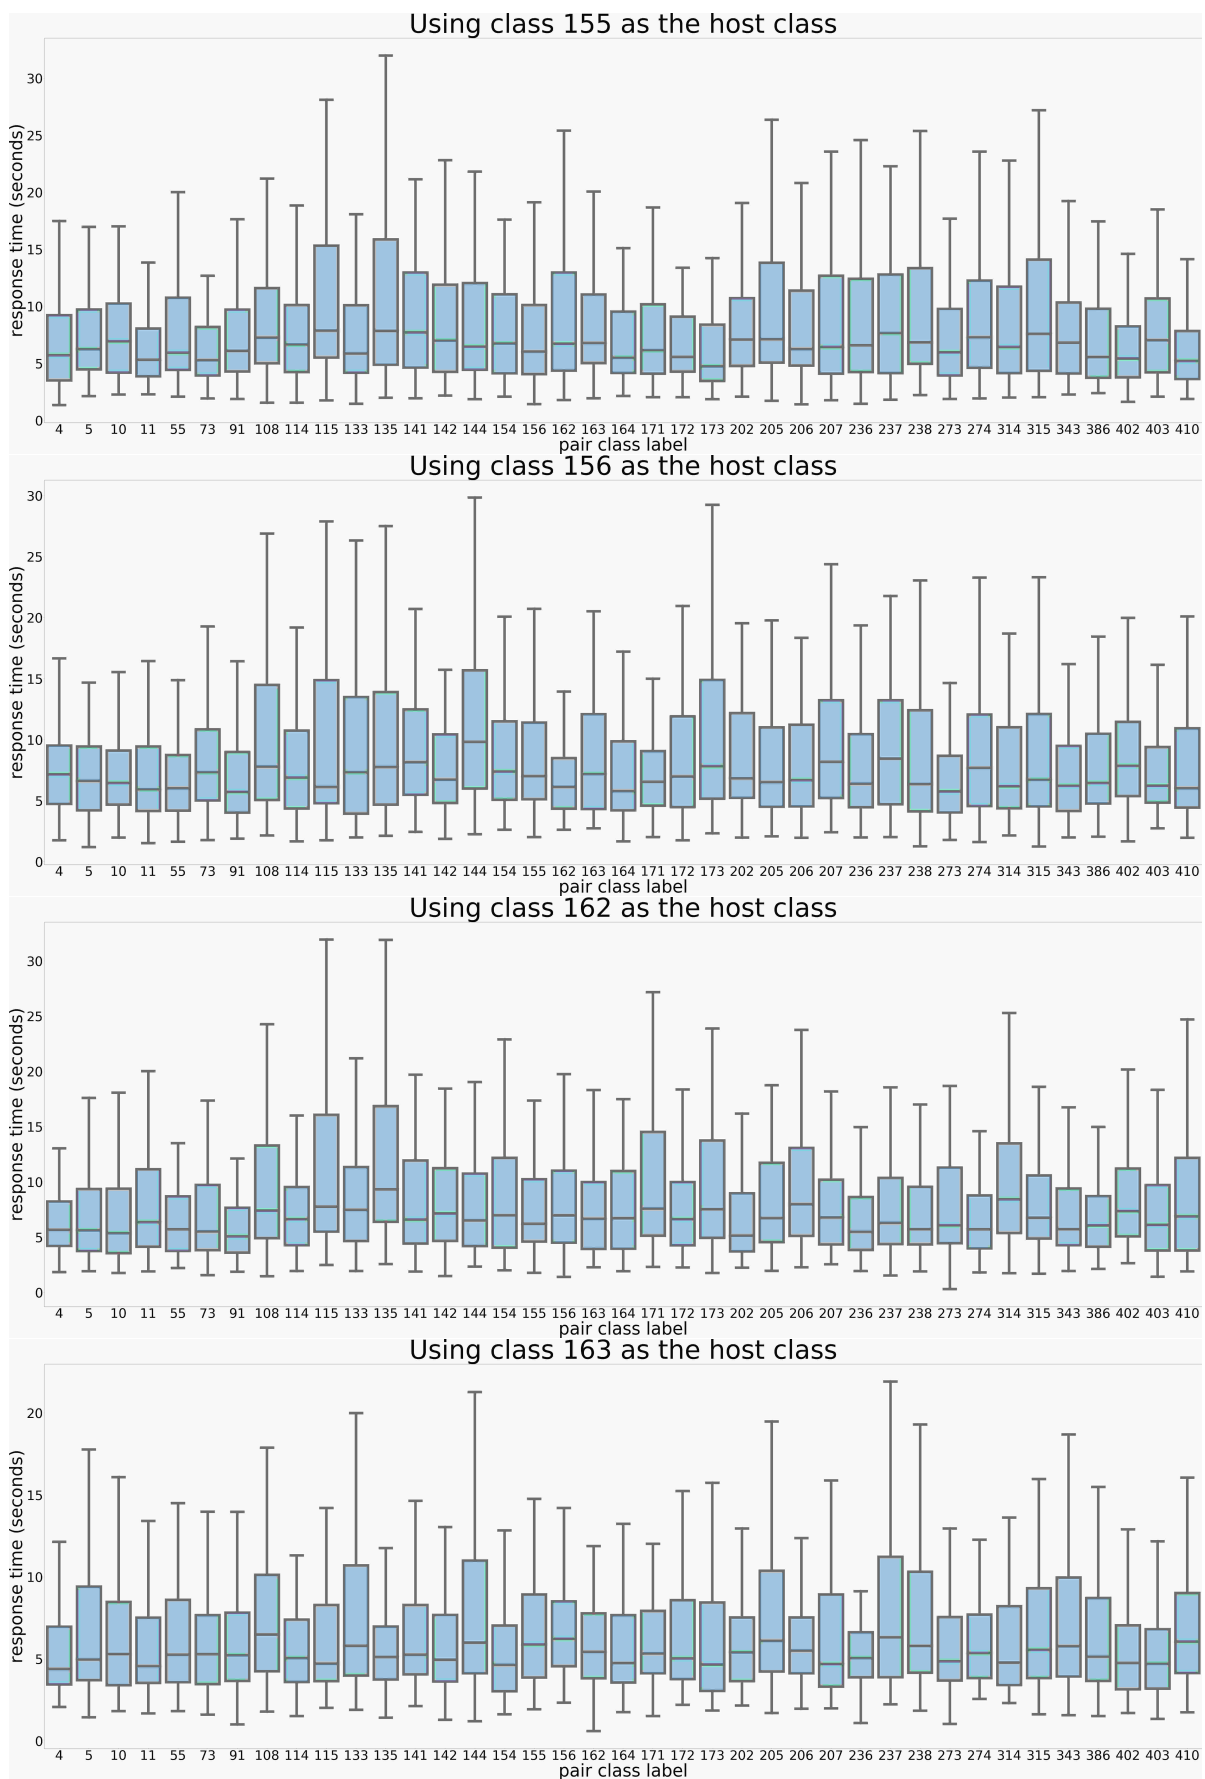

Figure 9: Using class 155, 156, 162 and 163 as the host class

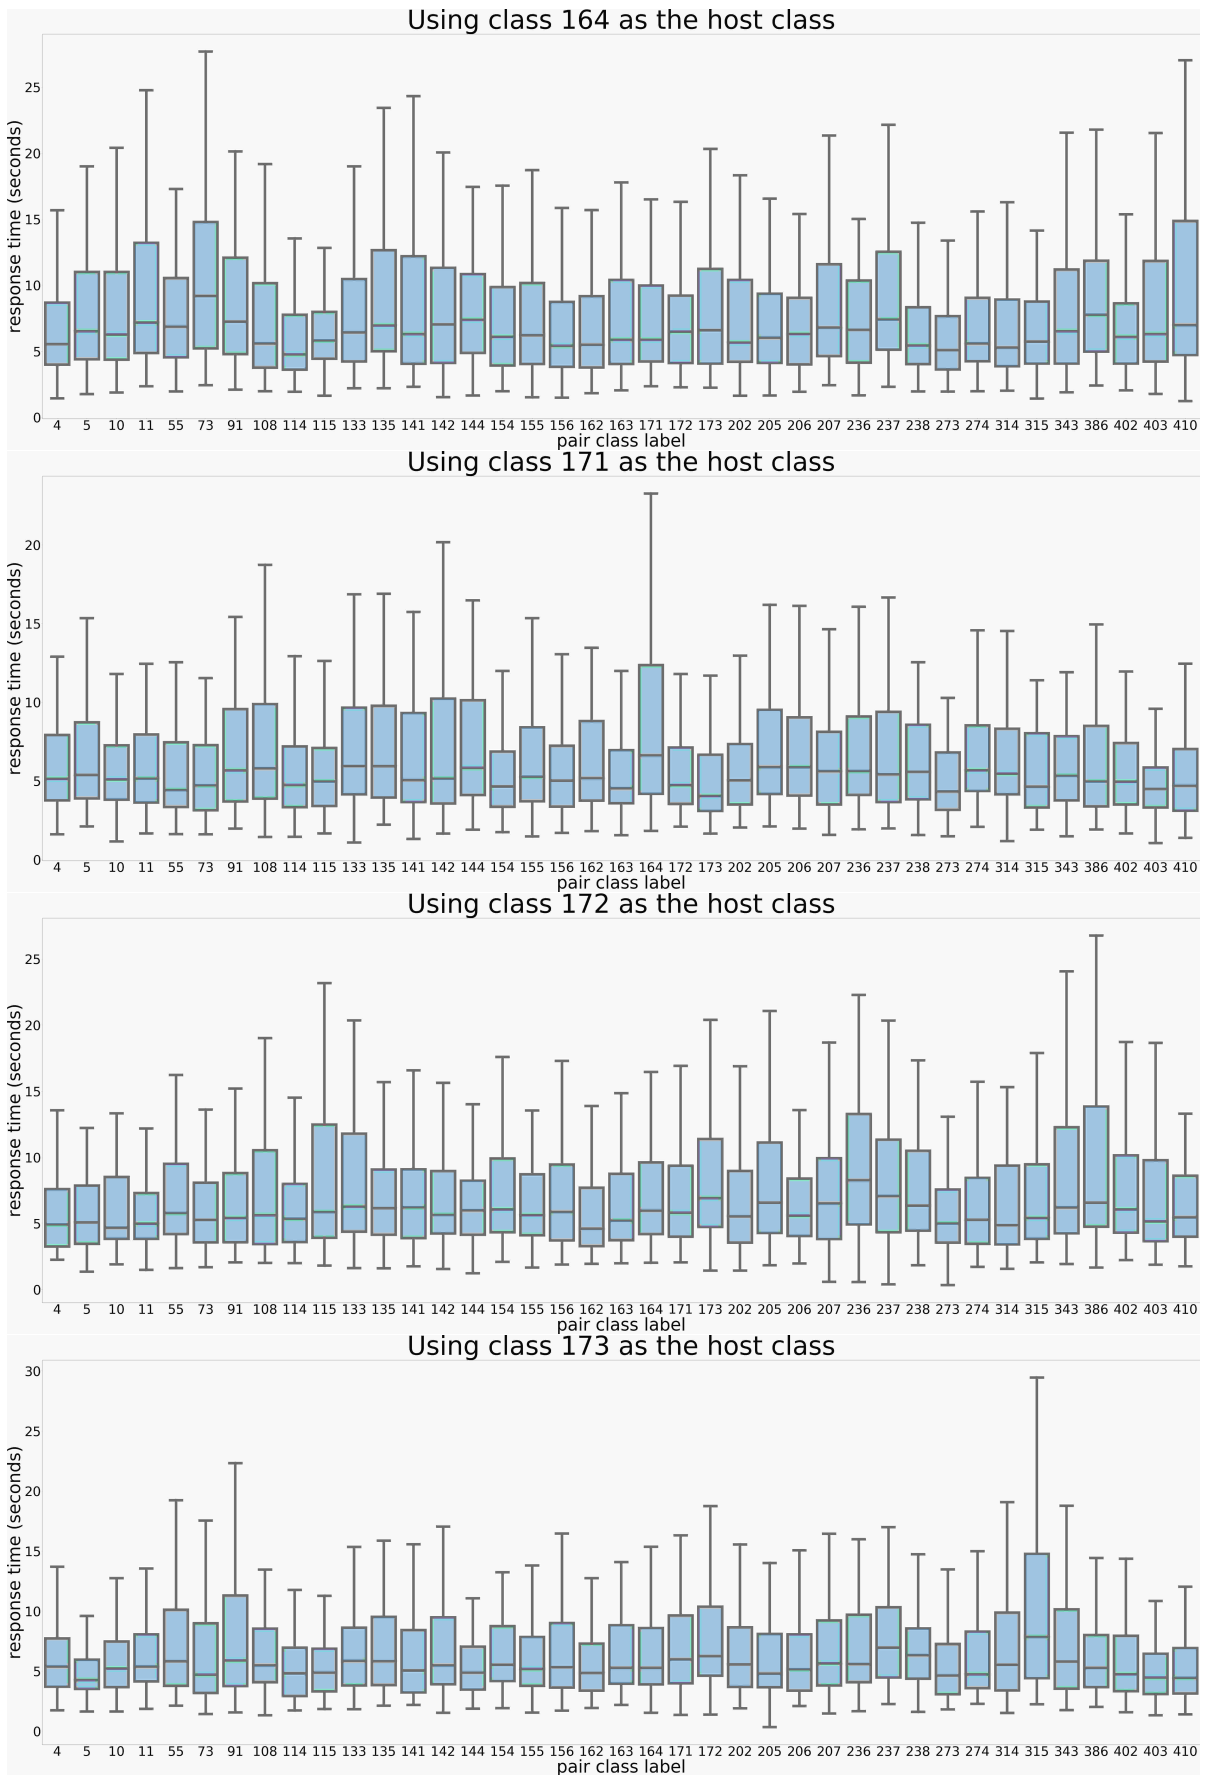

Figure 10: Using class 164, 171, 172 and 173 as the host class

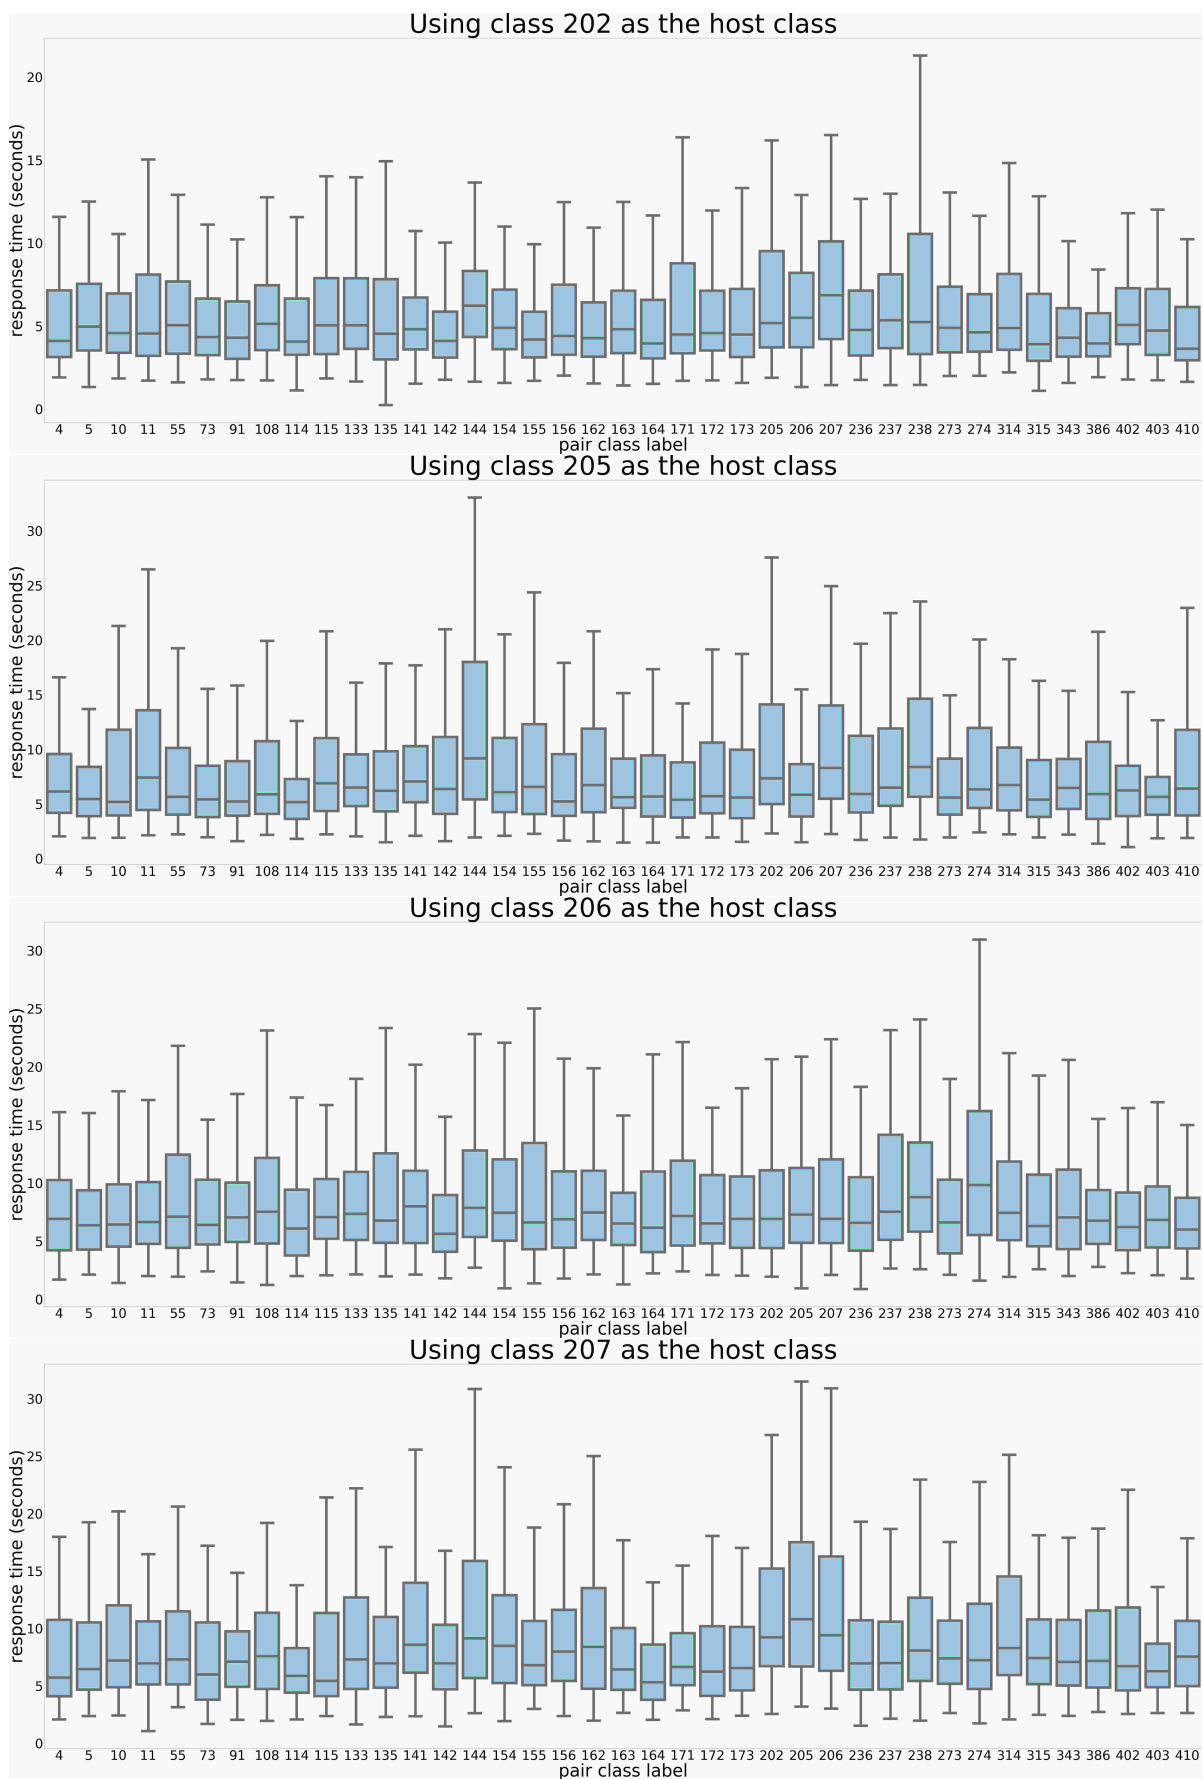

Figure 11: Using class 202, 205, 206, 207 as the host class

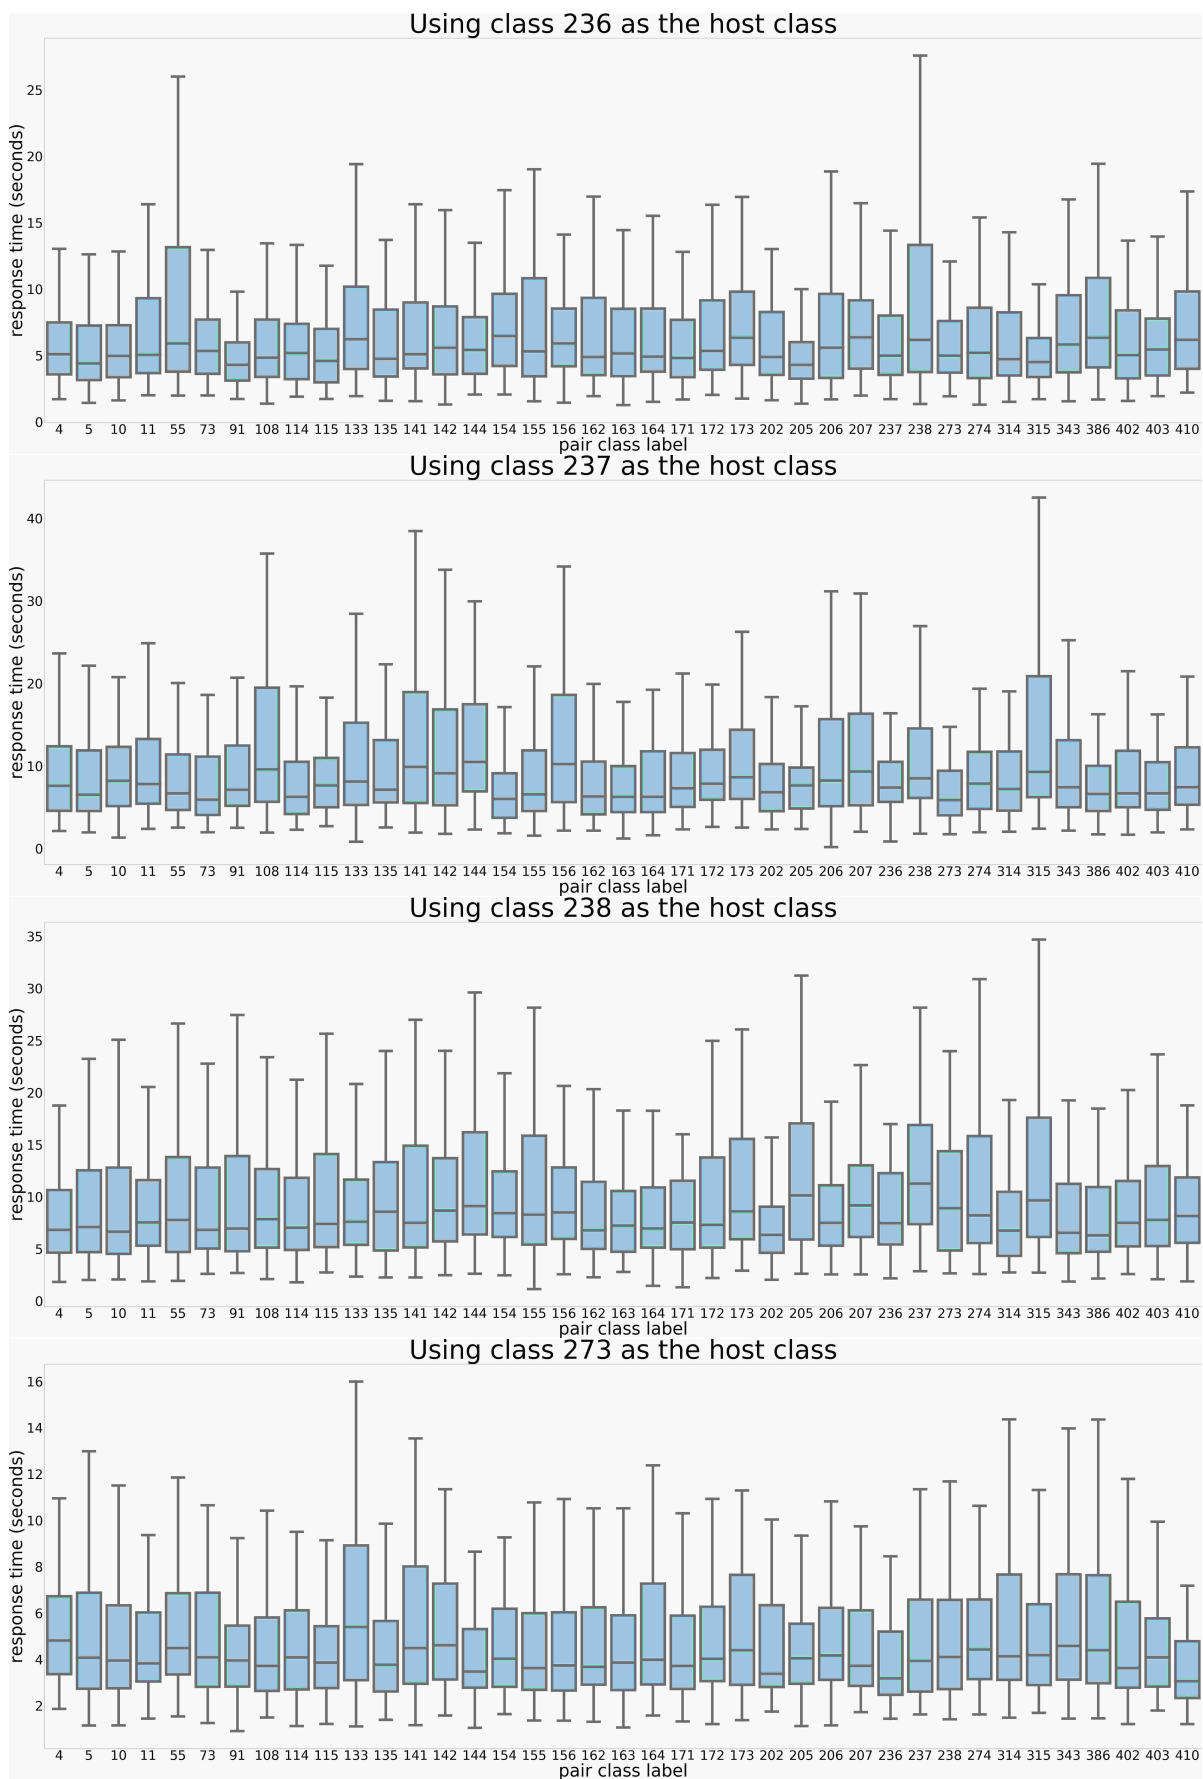

Figure 12: Using class 236, 237, 238, 273 as the host class

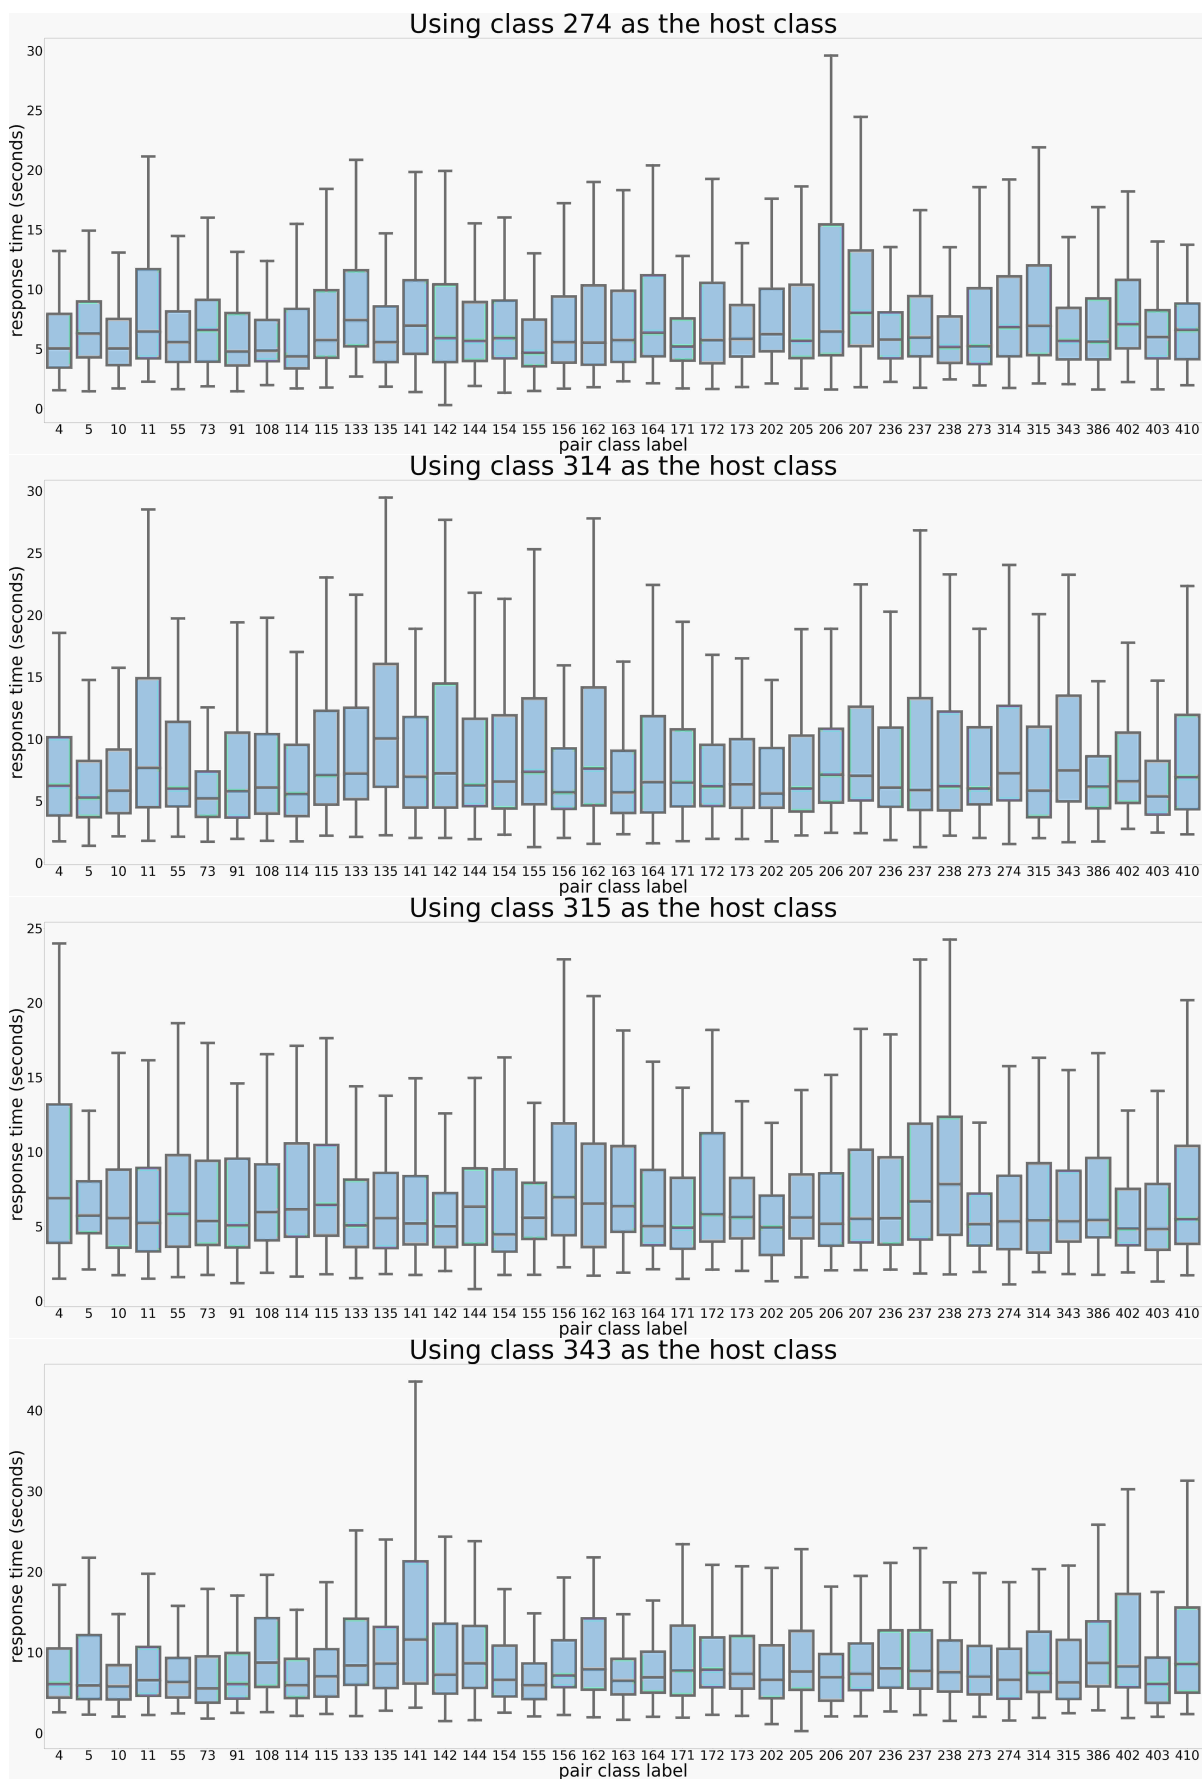

Figure 13: Using class 274, 314, 315, 343 as the host class

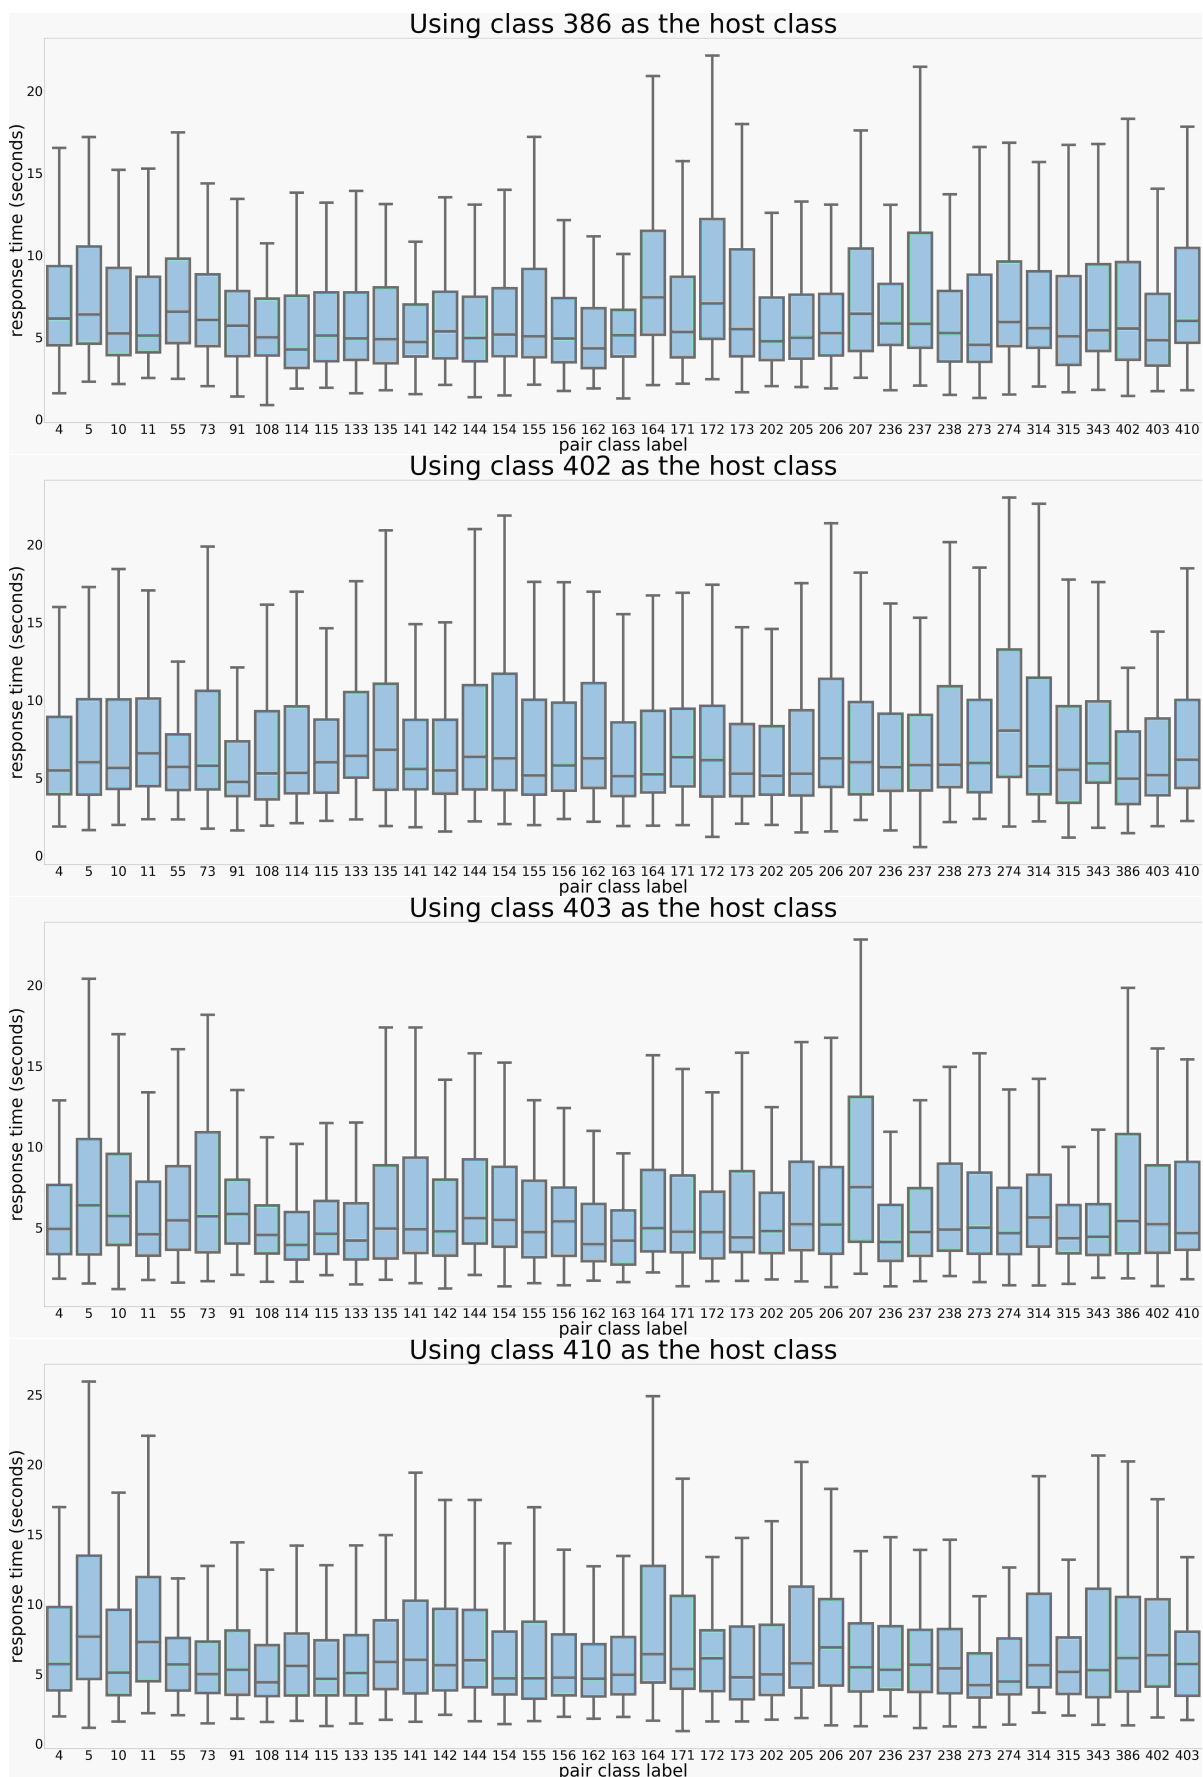

Figure 14: Using class 286, 402, 403, 410 as the host class

## 2 Descriptions of Baseline Approaches.

### 2.1 Standalone Classifiers

For the experiments involving standalone classifiers, we used the features that are generated by MSD-Net [1] when trained with the original Cross-Entropy loss on the ImageNet335 dataset. The SVM-based methods described below, as well as the EVM algorithm, were not originally designed to apply to feature sets of high dimensionality. When we use the original extracted features directly with these classifiers, the algorithms fail to converge due to the large number of dimensions. To address this issue, we utilized the Principal Component Analysis (PCA) method to reduce the size of features. To be specific, we first standardized features by removing the mean and scaling to unit variance using a standard scaler from scikit-learn (<https://scikit-learn.org/stable/modules/generated/sklearn.preprocessing.StandardScaler.html>). We then applied PCA to the standardized features such that the reduced features represented 99% of the original features. For the PCA algorithm, we used the implementation in scikit-learn (<https://scikit-learn.org/stable/modules/generated/sklearn.decomposition.IncrementalPCA.html?highlight=incremental+pca>) with a batch size of 512. Hyperparameters are set to implementation defaults unless otherwise mentioned.

To train the SVM, W-SVM,  $P_I$ -SVM and EVM, we fit the reduced features to each algorithm and obtained trained models. We then sent known samples with labels and unknown samples into the models, and obtained prediction scores. Last, we applied thresholding to each score to decide whether a sample is known or unknown. The threshold was obtained by calculating the median of predictions scores when passing the validation set through a trained model.

**SVM** [2] maps training samples into points in space so as to maximize the margin between different classes. It has been used in many applications in computer vision including, but not limited to, image classification, handwritten character recognition, and face recognition. Here we use the SVM implemented in scikit-learn and we apply the SGDClassifier (<https://scikit-learn.org/stable/modules/sgd.html?highlight=sgd>) to our features for simplicity. To be specific, we use the linear kernel with a  $C$  parameter of 1.

**Weibull-Calibrated SVM (W-SVM)** [3] introduces a Compact Abating Probability (CAP) model to tackle the OSR problem. In the proposed CAP model, the probability of being associated with a class decreases in value when a point moves from known to unknown space. Based on the CAP model, the authors propose a novel Weibull-calibrated SVM (W-SVM) algorithm. The W-SVM utilizes the statistical Extreme Value Theory for score calibration with one-class and binary SVMs. The code that is used for the W-SVM is from <https://github.com/ljain2/libsvm-openset>.

**$P_I$ -SVM** [4] utilizes the intuition that an algorithm should be able to reject a large portion of unknown samples during the testing phase if known samples are accurately modeled during the training phase without overfitting. Based on this intuition, the  $P_I$ -SVM models positive training data with the statistical Extreme Value Theory to determine decision boundaries, and it also uses a threshold-based strategy to generate classification results. The code that is used for the  $P_I$ -SVM is from <https://github.com/ljain2/libsvm-openset>.

**EVM** [5] is a theoretically sound open set classifier. It is inspired by the concept of support vectors in SVM, and is modeled by measuring the distribution of sample half-distances relative to a reference point. During the training phase, the EVM trains a one-vs-rest model for each known class; during the testing phase, it generates prediction scores for each testing sample. The code used for the EVM is from [https://github.com/priyatelj/vast/tree/massive\\_memory\\_use](https://github.com/priyatelj/vast/tree/massive_memory_use). The EVM parameters used are as follows: tail size=1000, cover threshold=0.5, distance multiplier=1.0, distance metric=cosine and chunk size=200.

### 2.2 Deep Learning-Based Methods

Researchers have been exploring deep learning-bases methods for OSR problems for several years and have come up with different approaches. We compare our MSD-Net trained with the proposed psychophysical loss with the following methods:

**OpenMax** [6] is the first open set classifier that can be trained with a deep neural network. It utilizes the features produced by a deep network to compute a Mean Activation Vector (MAV) and the distances for MAVs. Then it trains a Weibull model using the MAVs and their corresponding distances. During the testing phase, the model produces a probability vector of length  $n + 1$ , where  $n$  is the number of known samples, and the last value in the vector indicates the probability for being an unknown sample.

To reproduce OpenMax using our dataset, we chose the model that had the best performance (evaluated by top-1 validation accuracy) while training MSD-Net with Cross-Entropy loss on the ImageNet335 dataset, and passed the training set and testing set (both known and unknown) to the model to obtain features for each sample. Then we followed the pipeline implemented in <https://github.com/abhi jitbendale/OSDN> to calculate MAVs, distances of MAVs, and to train the Weibull model. Lastly we used the trained Weibull model to test all of our samples. The class that has the largest probability is considered to be the classification result.

**OSRCI** [7] generates samples that are close to training samples yet do not belong to any training class, using Generative Adversarial Networks. It trains a network that can classify these generated images into an extra class; ideally, when tested with unknown images, these unknown samples should be classified into the extra class.

We used the code publicly provided by the authors (<https://github.com/lwneal/counterfactual-open-set>) and followed the instructions step-by-step to apply this method to our ImageNet335 data. Parameter-wise, we randomly generated 50 batches of fake images, where each batch contained 64 images, which made 3,200 fake images in total. The network was trained for 200 epochs on a single GPU. After training, we evaluated the model with both known and unknown samples in the testing set, deciding what class a sample belonged to by looking at the class that had the largest prediction score.

**CROSR** [8] uses latent representations for reconstruction to enhance a model’s ability to learn known features and separate them from unknown samples. The method consists of a closed set classifier and an unknown detector, where the closed set classifier directly uses the target labels, and the unknown detector uses a reconstructive latent representation together with target labels.

We utilized the code from <https://github.com/saketd403/CROSR> to reproduce this method with our ImageNet335 data. We train CROSR for 200 epochs on a single GPU with a batch size of 16 and image size of 32, with an initial learning rate of 0.05, a momentum of 0.9, and a weight decay of 0.0005. After training, we found the best model by looking at the top-1 validation accuracy, and used that model for testing. Similar to the original paper, we used thresholding on the probability scores we obtained from testing samples to separate known and unknown samples; but instead of using a naive threshold of 0.5, we used the median of the probability scores obtained by using the validation data.

**CAC-OSR** [9] is a distance-based loss that trains known classes to form clusters around anchored class centers in the feature space, which makes it easier to distinguish known samples and unknown samples. It consists of a closed set classifier (which can be any existing network), a non-trainable parameter  $C$  that represents a set of class center points, and a new layer designed for the new loss.

Following the code provided at <https://github.com/dimitymiller/cac-openset>, we reproduce this method with our ImageNet335 data. We trained the model for 200 epochs, with a batch size of 64, and image size of 64. After training, we found the best model by looking at the top-1 validation accuracy, and used that model for testing. We calculated the median of the probability scores gained by the validation data, and used it as a threshold on the probability scores we obtained from testing samples to separate known and unknown classes.

### 3 Additional Tables (Experimental Details and Results)

Table 2 shows the cut-off thresholds that map bins of RT measurements to the MSD-Net exit indices, mentioned in Section IV of the main paper. The maximum is obtained by finding the largest value of RT after removing the outliers.

Table 3 shows the full breakdown of results (*i.e.*, the individual results for each of the 5 seeds) for the standalone classifier baselines, and Table 4 shows the full breakdown of results for the deep learning-based methods. The results in bold represent the best result for a specific metric among the 5 seeds for that method.

In Table 4, some values are “nan” for the Matthews correlation coefficient (MCC) score, because this metric is defined by:

$$MCC = \frac{TN \times TP - FN \times FP}{\sqrt{(TP + FP)(TP + FN)(TN + FP)(TN + FN)}} \quad (1)$$

When  $TN + FN$  is zero, the numerator in the equation is divided by zero, and thus leads to “not a number” as the result.

| Threshold     | QU1    | QU2    | QU3    | QU4    | Max    |
|---------------|--------|--------|--------|--------|--------|
| Percent Below | 20%    | 40%    | 60%    | 80%    | 100%   |
| Reaction Time | 3.5720 | 4.9740 | 7.0156 | 11.601 | 27.572 |
| Exit Index    | 0      | 1      | 2      | 3      | 4      |

Table 2: The cut-off thresholds for human RT for known samples. This table maps RT bins to the MSD-Net exit indices. The minimum is set to 0, and the other 5 thresholds are the quintiles (QU). All the values for reaction time are in seconds.

We also conducted a series of experiments for the four methods that utilized features that were reduced in dimensionality by PCA in order to explore algorithm sensitivity to different PCA settings. Recall from above that we applied PCA such that the reduced features represented 99% of the original features. In these experiments, we picked three larger fixed feature sizes that are reasonable for balancing information content and available computational resources: 250, 500 and 1000 dimensions. The corresponding results are shown in Table 5, Table 6 and Table 7. As can be seen, there is barely any change in the results, which indicates that our chosen dimensionality reduction scheme is reasonable, since increasing the dimensionality does not provide additional information. It is worth mentioning that after increasing the dimensionality, the EVM cannot detect known samples anymore and classifies every test sample as unknown. We use dashed lines to indicate this in the following tables.

## References

- [1] G. Huang, D. Chen, T. Li, F. Wu, L. van der Maaten, and K. Q. Weinberger, “Multi-scale dense networks for resource efficient image classification,” in *ICLR*, 2018.
- [2] C. Cortes and V. Vapnik, “Support-vector networks,” *Machine Learning*, vol. 20, no. 3, 1995.
- [3] W. J. Scheirer, L. P. Jain, and T. E. Boulton, “Probability models for open set recognition,” *IEEE T-PAMI*, vol. 36, no. 11, 2014.
- [4] L. P. Jain, W. J. Scheirer, and T. E. Boulton, “Multi-class open set recognition using probability of inclusion,” in *ECCV*, 2014.
- [5] E. M. Rudd, L. P. Jain, W. J. Scheirer, and T. E. Boulton, “The extreme value machine,” *IEEE T-PAMI*, vol. 40, no. 3, 2018.
- [6] A. Bendale and T. E. Boulton, “Towards Open Set Deep Networks,” in *Proceedings of the IEEE Conference on Computer Vision and Pattern Recognition*, 2016, pp. 1563–1572. [Online]. Available: [https://www.cv-foundation.org/openaccess/content\\_cvpr\\_2016/html/Bendale\\_Towards\\_Open\\_Set\\_CVPR\\_2016\\_paper.html](https://www.cv-foundation.org/openaccess/content_cvpr_2016/html/Bendale_Towards_Open_Set_CVPR_2016_paper.html)
- [7] L. Neal, M. Olson, X. Fern, W.-K. Wong, and F. Li, “Open set learning with counterfactual images,” in *ECCV*, 2018.
- [8] R. Yoshihashi, W. Shao, R. Kawakami, S. You, M. Iida, and T. Naemura, “Classification-reconstruction learning for open-set recognition,” in *IEEE/CVF CVPR*, 2019.
- [9] D. Miller, N. Sunderhauf, M. Milford, and F. Dayoub, “Class anchor clustering: A loss for distance-based open set recognition,” in *IEEE/CVF WACV*, 2021.

| Algorithm | Seed | TP            | TN           | FP           | FN            | F-1           | MCC            | Test Unknown  | Test Known Top-1 |
|-----------|------|---------------|--------------|--------------|---------------|---------------|----------------|---------------|------------------|
| SVM       | 0    | <b>164378</b> | 25599        | 22468        | <b>172070</b> | <b>0.6282</b> | 0.0139         | 0.5326        | 0.0062           |
|           | 1    | 163091        | <b>27448</b> | <b>20619</b> | 173357        | 0.6271        | <b>0.0369</b>  | <b>0.5710</b> | 0.0041           |
|           | 2    | 154708        | 26632        | 21435        | 181740        | 0.6036        | 0.0092         | 0.5541        | 0.0046           |
|           | 3    | 151932        | 25628        | 22439        | 184516        | 0.5949        | -0.0101        | 0.5332        | 0.0067           |
|           | 4    | 152100        | 26984        | 21083        | 184348        | 0.5969        | 0.00894        | 0.5614        | <b>0.0082</b>    |
| W-SVM     | 0    | 350           | 0            | 48087        | 336078        | 0.0018        | -0.9959        | 0.0923        | 0.0009           |
|           | 1    | 381           | 0            | 47931        | 336203        | <b>0.0020</b> | -0.9955        | 0.0934        | 0.0010           |
|           | 2    | 362           | 0            | 48115        | 336038        | 0.0019        | -0.9957        | 0.0928        | 0.0009           |
|           | 3    | <b>410</b>    | 0            | <b>47101</b> | 337004        | 0.0021        | <b>-0.9951</b> | <b>0.1101</b> | <b>0.0011</b>    |
|           | 4    | 392           | 0            | 48112        | <b>336011</b> | <b>0.0020</b> | -0.9954        | 0.0981        | 0.0010           |
| Pi-SVM    | 0    | <b>891</b>    | 201          | 48066        | <b>335357</b> | <b>0.0046</b> | <b>-0.9872</b> | 0.0832        | <b>0.0028</b>    |
|           | 1    | 807           | 208          | 48121        | 335379        | 0.0042        | -0.9881        | 0.0810        | 0.0026           |
|           | 2    | 851           | 210          | 48010        | 335444        | 0.0044        | -0.9875        | 0.0827        | <b>0.0028</b>    |
|           | 3    | 790           | 240          | <b>48001</b> | 335484        | 0.0041        | -0.9879        | <b>0.0851</b> | 0.0027           |
|           | 4    | 830           | <b>247</b>   | 48057        | 335381        | 0.0043        | -0.9873        | 0.0832        | <b>0.0028</b>    |
| OpenMax   | 0    | 187520        | 19882        | 28182        | 132576        | 0.7000        | -0.0004        | 0.4137        | 0.0036           |
|           | 1    | 226722        | 13591        | 34473        | 94014         | 0.7792        | -0.0077        | 0.2828        | 0.0037           |
|           | 2    | <b>249973</b> | 9967         | 38097        | 69771         | <b>0.8225</b> | -0.0089        | 0.2074        | <b>0.0047</b>    |
|           | 3    | 189123        | <b>20942</b> | <b>27122</b> | 132893        | 0.7027        | <b>0.0157</b>  | <b>0.4357</b> | 0.0034           |
|           | 4    | 228974        | 13520        | 34544        | <b>91346</b>  | 0.7844        | -0.0029        | 0.2813        | 0.0040           |
| EVM       | 0    | 1977          | 47796        | 271          | 334471        | 0.0117        | 0.0010         | 0.9944        | 0.0047           |
|           | 1    | 1293          | 47870        | 197          | 335155        | 0.0077        | -0.0014        | 0.9959        | 0.0036           |
|           | 2    | 1142          | <b>47918</b> | <b>149</b>   | 335306        | 0.0068        | 0.0017         | <b>0.9969</b> | 0.0035           |
|           | 3    | 1952          | 47812        | 255          | 334496        | 0.0115        | <b>0.0022</b>  | 0.9947        | 0.0050           |
|           | 4    | <b>3602</b>   | 47494        | 573          | <b>332846</b> | <b>0.0211</b> | -0.0039        | 0.9881        | <b>0.0061</b>    |

Table 3: Testing results for standalone classifier baselines.

| Algorithm         | Seed | TP            | TN           | FP           | FN            | F-1           | MCC           | Test Unknown  | Test Known Top-1 |
|-------------------|------|---------------|--------------|--------------|---------------|---------------|---------------|---------------|------------------|
| OSRCI             | 0    | 336179        | 39           | 48025        | 205           | 0.9330        | 0.0027        | 0.0008        | <b>0.0040</b>    |
|                   | 1    | <b>336384</b> | 0            | 48064        | <b>0</b>      | 0.9333        | nan           | 0             | 0.0038           |
|                   | 2    | 321613        | <b>2052</b>  | <b>46012</b> | 14771         | 0.9137        | -0.0020       | <b>0.0427</b> | 0.0030           |
|                   | 3    | <b>336384</b> | 0            | 48064        | <b>0</b>      | <b>0.9333</b> | nan           | 0             | 0.0037           |
|                   | 4    | 332311        | 581          | 47483        | 4073          | 0.9280        | -0.0001       | 0.0121        | 0.0036           |
| CROSR             | 0    | 54089         | 41069        | 6995         | 282295        | 0.2722        | 0.0138        | 0.8545        | 0.0205           |
|                   | 1    | 50193         | 41568        | 6496         | 286191        | 0.2554        | 0.0131        | 0.8648        | 0.0174           |
|                   | 2    | <b>56809</b>  | 40773        | 7291         | <b>279575</b> | <b>0.2837</b> | 0.0153        | 0.8483        | <b>0.0209</b>    |
|                   | 3    | 54324         | 41114        | 6950         | 282108        | 0.2732        | 0.0152        | 0.8554        | 0.0201           |
|                   | 4    | 51308         | <b>41625</b> | <b>6439</b>  | 285076        | 0.2604        | <b>0.0172</b> | <b>0.8660</b> | 0.0174           |
| CAC-OSR           | 0    | 21776         | 45255        | 2809         | 314608        | 0.1207        | 0.0085        | 0.9416        | 0.0005           |
|                   | 1    | 20999         | <b>45569</b> | <b>2495</b>  | 315385        | 0.1167        | 0.0145        | <b>0.9481</b> | 0.0004           |
|                   | 2    | 20825         | 45546        | 2518         | 315559        | 0.1158        | 0.0132        | 0.9476        | 0.0005           |
|                   | 3    | <b>22820</b>  | 45366        | 2698         | <b>313564</b> | <b>0.1261</b> | <b>0.0156</b> | 0.9439        | <b>0.0006</b>    |
|                   | 4    | 20008         | 45498        | 2566         | 316376        | 0.1114        | 0.0086        | 0.9466        | 0.0005           |
| $Loss_C$          | 0    | 335697        | 9616         | 38448        | 735           | 0.9449        | 0.4043        | 0.2000        | 0.2198           |
|                   | 1    | 335787        | 9744         | 38320        | 648           | 0.9452        | 0.4095        | 0.2027        | 0.3244           |
|                   | 2    | <b>335928</b> | <b>11039</b> | <b>37025</b> | <b>520</b>    | <b>0.9471</b> | <b>0.4418</b> | <b>0.2297</b> | <b>0.3785</b>    |
|                   | 3    | 335811        | 9558         | 38506        | 622           | 0.9449        | 0.4058        | 0.1989        | 0.2615           |
|                   | 4    | 335830        | 10646        | 37418        | 605           | 0.9464        | 0.4311        | 0.2215        | 0.3260           |
| $Loss_C + Loss_P$ | 0    | 335587        | 8891         | 39173        | 846           | 0.9437        | 0.3841        | 0.1850        | 0.2673           |
|                   | 1    | 335419        | <b>17034</b> | <b>31033</b> | 1029          | <b>0.9544</b> | <b>0.5491</b> | <b>0.3544</b> | <b>0.3932</b>    |
|                   | 2    | <b>335801</b> | 10605        | 37459        | <b>634</b>    | 0.9463        | 0.4295        | 0.2206        | 0.3359           |
|                   | 3    | 335739        | 9798         | 38266        | 694           | 0.9452        | 0.4096        | 0.2039        | 0.2595           |
|                   | 4    | 335667        | 11237        | 36827        | 768           | 0.9470        | 0.4402        | 0.2338        | 0.3426           |
| Proposed          | 0    | 335565        | 26312        | 21755        | 883           | 0.9674        | 0.7028        | 0.5474        | 0.4014           |
|                   | 1    | 335520        | <b>26814</b> | <b>21253</b> | 928           | <b>0.9680</b> | <b>0.7095</b> | <b>0.5578</b> | <b>0.4052</b>    |
|                   | 2    | 335601        | 25866        | 22201        | 847           | 0.9668        | 0.6967        | 0.5381        | 0.3931           |
|                   | 3    | <b>335654</b> | 25949        | 22118        | <b>794</b>    | 0.9670        | 0.6988        | 0.5399        | 0.3933           |
|                   | 4    | 335559        | 25415        | 22652        | 889           | 0.9661        | 0.6892        | 0.5287        | 0.3905           |

Table 4: Testing results for deep learning-based baselines.

| Algorithm | Seed | TP            | TN          | FP           | FN            | F-1           | MCC            | Test Unknown  | Test Known Top-1 |
|-----------|------|---------------|-------------|--------------|---------------|---------------|----------------|---------------|------------------|
| SVM       | 0    | 156428        | 1519        | 1485         | 180020        | 0.6328        | -0.0055        | 0.5057        | 0.0060           |
|           | 1    | <b>159912</b> | 1608        | 1396         | <b>176536</b> | <b>0.6425</b> | <b>0.0020</b>  | 0.5352        | 0.0041           |
|           | 2    | 152790        | 1578        | 1426         | 183658        | 0.6228        | -0.004         | 0.5252        | 0.0042           |
|           | 3    | 146332        | 1527        | 1477         | 190116        | 0.6044        | -0.0107        | 0.5083        | 0.0069           |
|           | 4    | 143729        | <b>1645</b> | <b>1359</b>  | 192719        | 0.5969        | -0.0048        | <b>0.5476</b> | <b>0.0079</b>    |
| W-SVM     | 0    | 320           | 0           | 51021        | 333165        | 0.0017        | -0.9964        | 0.0911        | 0.0008           |
|           | 1    | 331           | 0           | 51321        | <b>332855</b> | 0.0017        | -0.9963        | 0.0914        | <b>0.0009</b>    |
|           | 2    | 315           | 0           | 50206        | 333985        | <b>0.0016</b> | -0.9964        | 0.0910        | 0.0008           |
|           | 3    | <b>341</b>    | 0           | 49985        | 334180        | 0.0018        | <b>-0.9961</b> | 0.0921        | <b>0.0009</b>    |
|           | 4    | 334           | 0           | <b>49912</b> | 334260        | 0.0017        | -0.9962        | <b>0.0929</b> | <b>0.0009</b>    |
| Pi-SVM    | 0    | 721           | 189         | <b>48210</b> | 335386        | 0.0037        | -0.9892        | 0.0821        | 0.0024           |
|           | 1    | 744           | <b>211</b>  | 48328        | 335223        | 0.0039        | -0.9891        | 0.0839        | 0.0025           |
|           | 2    | 721           | 205         | 48290        | 335290        | 0.0037        | <b>-0.9889</b> | 0.0829        | 0.0024           |
|           | 3    | 749           | 188         | 48381        | <b>335188</b> | 0.0039        | -0.9892        | <b>0.0864</b> | 0.0024           |
|           | 4    | <b>812</b>    | 201         | 48922        | 334571        | <b>0.0042</b> | -0.9891        | 0.0821        | <b>0.0026</b>    |
| EVM       | 0    | -             | -           | -            | -             | -             | -              | -             | -                |
|           | 1    | -             | -           | -            | -             | -             | -              | -             | -                |
|           | 2    | -             | -           | -            | -             | -             | -              | -             | -                |
|           | 3    | -             | -           | -            | -             | -             | -              | -             | -                |
|           | 4    | -             | -           | -            | -             | -             | -              | -             | -                |

Table 5: Testing results for the four methods that use features after the application of PCA to reduce the representation to 250 dimensions.

| Algorithm | Seed | TP            | TN          | FP           | FN            | F-1           | MCC            | Test Unknown  | Test Known Top-1 |
|-----------|------|---------------|-------------|--------------|---------------|---------------|----------------|---------------|------------------|
| SVM       | 0    | 146845        | 1602        | 1402         | 189603        | 0.6059        | -0.0057        | 0.5332        | 0.0062           |
|           | 1    | <b>151455</b> | 1666        | 1338         | <b>184993</b> | <b>0.6191</b> | <b>0.0008</b>  | 0.5545        | 0.0040           |
|           | 2    | 144019        | 1663        | 1341         | 192429        | 0.5978        | -0.0034        | 0.5535        | 0.0048           |
|           | 3    | 146845        | 1602        | 1402         | 189603        | 0.6059        | -0.0057        | 0.5332        | 0.0062           |
|           | 4    | 133415        | <b>1703</b> | <b>1301</b>  | 203033        | 0.5663        | -0.0069        | <b>0.5669</b> | <b>0.0081</b>    |
| W-SVM     | 0    | 298           | 0           | 52012        | <b>332196</b> | 0.0015        | -0.9967        | <b>0.0899</b> | 0.0008           |
|           | 1    | 310           | 0           | 51882        | 332314        | <b>0.0016</b> | -0.9966        | 0.0891        | 0.0008           |
|           | 2    | 305           | 0           | 51841        | 332860        | <b>0.0016</b> | -0.9966        | 0.0887        | 0.0008           |
|           | 3    | 310           | 0           | <b>51202</b> | 332994        | <b>0.0016</b> | <b>-0.9965</b> | 0.0881        | 0.0008           |
|           | 4    | <b>330</b>    | 0           | 51303        | 332873        | <b>0.0016</b> | <b>-0.9965</b> | 0.0881        | 0.0008           |
| Pi-SVM    | 0    | 751           | <b>228</b>  | 50092        | 333435        | 0.0039        | -0.9891        | 0.0812        | 0.0025           |
|           | 1    | 758           | 221         | 50101        | 333426        | 0.0039        | <b>-0.9890</b> | 0.0814        | 0.0025           |
|           | 2    | <b>763</b>    | 211         | <b>50085</b> | 333447        | <b>0.0040</b> | -0.9892        | 0.0819        | 0.0024           |
|           | 3    | 755           | 226         | 51012        | 332513        | 0.0039        | -0.9891        | <b>0.0825</b> | <b>0.0026</b>    |
|           | 4    | 758           | 222         | 51018        | <b>332508</b> | 0.0039        | -0.9892        | 0.0821        | 0.0025           |
| EVM       | 0    | -             | -           | -            | -             | -             | -              | -             | -                |
|           | 1    | -             | -           | -            | -             | -             | -              | -             | -                |
|           | 2    | -             | -           | -            | -             | -             | -              | -             | -                |
|           | 3    | -             | -           | -            | -             | -             | -              | -             | -                |
|           | 4    | -             | -           | -            | -             | -             | -              | -             | -                |

Table 6: Testing results for the four methods that use features after the application of PCA to reduce the representation to 500 dimensions.

| Algorithm | Seed | TP            | TN          | FP           | FN            | F-1           | MCC            | Test Unknown  | Test Known Top-1 |
|-----------|------|---------------|-------------|--------------|---------------|---------------|----------------|---------------|------------------|
| SVM       | 0    | 135028        | 1737        | <b>1267</b>  | 201420        | 0.5712        | -0.0039        | 0.5782        | 0.0067           |
|           | 1    | <b>139877</b> | 1745        | 1259         | 196571        | <b>0.5857</b> | <b>-0.0006</b> | 0.5808        | 0.0039           |
|           | 2    | 132666        | 1748        | 1256         | 203782        | 0.5640        | -0.0045        | 0.5818        | 0.0045           |
|           | 3    | 135028        | 1737        | <b>1267</b>  | 201420        | 0.5712        | -0.0039        | 0.5782        | 0.0067           |
|           | 4    | 121726        | <b>1815</b> | 1189         | <b>214722</b> | 0.5299        | -0.0066        | <b>0.6041</b> | <b>0.0084</b>    |
| W-SVM     | 0    | 280           | 0           | 53292        | 330934        | <b>0.0015</b> | -0.9970        | 0.0812        | 0.0007           |
|           | 1    | <b>288</b>    | 0           | 53288        | <b>330930</b> | <b>0.0015</b> | <b>-0.9969</b> | 0.0822        | 0.0007           |
|           | 2    | 276           | 0           | <b>53197</b> | 331033        | 0.0014        | -0.9970        | 0.0821        | 0.0007           |
|           | 3    | 275           | 0           | 53229        | 331002        | 0.0014        | -0.9979        | <b>0.0827</b> | 0.0007           |
|           | 4    | 281           | 0           | 53212        | 331013        | <b>0.0015</b> | <b>-0.9969</b> | 0.0821        | 0.0007           |
| Pi-SVM    | 0    | 731           | 235         | <b>51241</b> | 332299        | 0.0038        | -0.9892        | 0.0808        | 0.0025           |
|           | 1    | 735           | 240         | 51255        | 332276        | 0.0038        | -0.9891        | 0.0812        | 0.0025           |
|           | 2    | 744           | <b>252</b>  | 51265        | <b>332245</b> | <b>0.0039</b> | <b>-0.9889</b> | 0.0818        | 0.0024           |
|           | 3    | <b>750</b>    | 243         | 51254        | 332259        | <b>0.0039</b> | <b>-0.9889</b> | 0.0815        | <b>0.0026</b>    |
|           | 4    | 753           | 247         | 51259        | 332247        | <b>0.0039</b> | <b>-0.9889</b> | <b>0.0816</b> | <b>0.0026</b>    |
| EVM       | 0    | -             | -           | -            | -             | -             | -              | -             | -                |
|           | 1    | -             | -           | -            | -             | -             | -              | -             | -                |
|           | 2    | -             | -           | -            | -             | -             | -              | -             | -                |
|           | 3    | -             | -           | -            | -             | -             | -              | -             | -                |
|           | 4    | -             | -           | -            | -             | -             | -              | -             | -                |

Table 7: Testing results for the four methods that use features after the application of PCA to reduce the representation to 1000 dimensions.
